# Supplementary material for: On The (In)Effectiveness of Static Logic Bomb Detector for Android Apps
Source: arXiv:2108.10381 source file (2021-08-25)
Supplement: Supplementary file 1 [file overview.tex]

\begin{figure*}[h]
\centering
\input{tikz/overview_tsopen.tikz}
\caption{Overview of TSOpen. First, the application APK is processed by \textsc{Flowdroid} to model the application. Then, every step of the analysis is applied to the ICFG until the final decision of suspiciousness of the application is taken by our tool.}
\end{figure*}
